# Supplementary material for: Proto-CLIP: Vision-Language Prototypical Network for Few-Shot Learning
Source: arXiv:2307.03073 ancillary file (2024-07-14)
Supplement: Supplementary file 1 [file Proto_CLIP_supp.pdf]

# PROTO-CLIP: Vision-Language Prototypical Network for Few-Shot Learning [ Supplementary Material ]

**Jishnu Jaykumar P**[1] **Kamalesh Palanisamy**[1] **Yu-Wei Chao**[2] **Xinya Du**[1] **Yu Xiang**[1]
[1]The University of Texas at Dallas [2]NVIDIA
{jishnu.p,kamalesh.palanisamy,xinya.du,yu.xiang}@utdallas.edu, ychao@nvidia.com

## Contents

**1 Experiments** **2**

1.1 $NK$ Setup . . . . . . 2

1.2 Dataset Splits File . . . . . . 2

1.3 HyperParameters . . . . . . 2

**2 Extended Ablation Study** **4**

**3 t-SNE Plot** **4**

**4 Real-World-Testing as in FEWSOL [1]** **5**

**5 Frequently Asked Questions (FAQ)** **6**

**6 A Study w.r.t. SAM [2]** **8**

# 1 Experiments

## 1.1 $NK$ Setup

Our research focuses on addressing the $N$-way $K$-shot classification problem, which involves the classification of data into $N$ classes using $K$ samples per class. In our approach, we organize the problem into episodes, with each episode comprising a set of $N$ classes and $K$ samples from each class. In contrast to the methodology employed in Tip-Adapter [2], where all classes are considered for episode composition, we adopt a random sampling technique for the selection of classes to form the episodes. This sampling protocol ensures that all the classes are encountered within a single epoch of the training process.

By incorporating random sampling of classes, we hope to enhance the diversity and generalizability of the training episodes. This technique ensures that the model encounters a wide range of classes during the training phase, facilitating better learning and improved performance on unseen data. By adopting a sophisticated sampling protocol and incorporating random class selection, our method demonstrates a robust and comprehensive approach to the $N$-way $K$-shot classification problem. Using diverse training episodes enhances the model's ability to generalize to new classes and improves its overall performance on various classification tasks.

## 1.2 Dataset Splits File

In accordance with the established practices set forth by Tip-Adapter [3], we adopted the identical splits file for our experimental analysis, encompassing a total of 11 datasets. Since, we want to improve object classification for robot manipulation tasks, FEWSOL [1] is one additional dataset that we have added to the pool of 11 datasets considered in Tip-Adapter [3] which is highly beneficial for few shot learning in robotic environments. This approach ensures a fair and meaningful comparison with the findings presented in Tip-Adapter [3] and FEWSOL [1], where an extensive investigation into the efficacy of CLIP [4] and its variants has been meticulously demonstrated.

A splits file serves as a crucial component, providing comprehensive information regarding the train/val/test split for each dataset. This information is instrumental in facilitating both the training and evaluation processes. We have created new splits file for 4 variants as in FEWSOL [1]: (i) FEWSOL-11 (ii) FEWSOL-41 (iii) FEWSOL-52 (iv) FEWSOL-198. The $C$ in FEWSOL-$C$ indicates the number of classes in the splits.

| **FEWSOL-C** | **Description** |
|---|---|
| FEWSOL-11 | Consists of 11 classes overlapping between synthetic 125 classes and real 198 classes |
| FEWSOL-41 | Consists of 41 classes which are not present in synthetic classes |
| FEWSOL-52 | Consists of union of FEWSOL-41 and FEWSOL-11 |
| FEWSOL-198 | Consists of all of the real classes with real world testing images as mentioned in Section. 4 |

Table 1: Description of 4 FEWSOL [1] dataset variants. We have considered FEWSOL-52 [1] and FEWSOL-198 [1] in our experiments. Splits file of each are shared with this work.

By adhering to the utilization of the same splits file, we strive to uphold the principles of reproducibility and promote a transparent and equitable comparison with previous methodologies.

We highly encourage the adoption of a similar mechanism in future research endeavors within this domain. Such adherence to consistent practices would not only contribute to the reproducibility of results but also foster a fair and valid comparison to previous methods. By aligning our methodologies, the scientific community can effectively build upon existing knowledge and drive the field forward in a robust and meaningful manner.

## 1.3 HyperParameters

The table provides a comprehensive overview of the hyperparameters considered in the PROTO-CLIP experiments. These hyperparameters play a crucial role in configuring and fine-tuning the model's

| Hyperparameter | Description |
|---|---|
| $\alpha$ | Controls the contribution from image and text memory bank |
| $\beta$ | Controls the sharpness of the logits. Acts like a temperature parameter as in [5] |
| $K$ | Shots to be considered for building the visual and textual memory bank |
| Train-Text-Memory | A boolean flag indicating whether to train text memory bank |
| Adapter | The alias of the available adapters in PROTO-CLIP: ['3xConv', '2xConv', 'MLP'] |
| Backbone | The alias of the available CLIP [4] backbones: ['RN50', 'RN101', 'ViT-B/16', 'ViT-B/32', 'ViT-L/14'] |

Table 2: Description of hyperparameters considered in PROTO-CLIP experiments.

behavior, allowing researchers to explore different settings and optimize its performance based on specific requirements and objectives.

$\boldsymbol{\alpha}$. This hyperparameter controls the contribution from the image and text memory bank. It determines the balance between visual and textual information during the classification process. By adjusting the value of $\alpha$, researchers can emphasize the importance of either modality, enabling the model to effectively leverage the strengths of both image and text representations.

$\boldsymbol{\beta}$. Acting as a sharpness control parameter, $\beta$ influences the logits' sharpness in the classification process. It functions similarly to a temperature parameter, as observed in the work of [5]. By manipulating $\beta$, researchers can control the spread of probabilities assigned to different classes, thus affecting the model's confidence levels in its predictions.

**Adapter.** The adapter hyperparameter refers to the alias of the available adapters in PROTO-CLIP. In the context of PROTO-CLIP, the framework offers a selection of adapters, each associated with a specific alias. The available aliases for the adapters are as follows: ['3xConv', '2xConv', 'MLP']. In the main paper, these aliases are further clarified and correspond to the following adapter configurations:

- 3xConv: This alias represents an adapter configuration consisting of three convolutional layers. Each layer applies a set of filters to the input data, enabling the model to extract and learn relevant features through hierarchical transformations. The '3xConv' adapter offers increased expressive power and potential for capturing intricate patterns within the data.
- 2xConv: This alias denotes an adapter configuration comprising two convolutional layers. Similar to the '3xConv' adapter, the '2xConv' adapter utilizes convolutional operations to extract meaningful features from the input data. Although it has a slightly simpler architecture than the '3xConv' adapter, the '2xConv' adapter still maintains a notable capacity for capturing and representing essential characteristics of the data.
- MLP: The 'MLP' alias refers to the adapter configuration known as MLP, which stands for Multi-Layer Perceptron. The MLP adapter consists of one hidden layer with a size equal to $D/4$, where $D$ represents the embedding size derived from the CLIP backbone. The MLP adapter employs fully connected layers, allowing for non-linear transformations and the integration of complex interactions between the input features.

By leveraging these different adapter configurations, researchers can tailor the behavior of PROTO-CLIP to their specific needs and experiment with various levels of model complexity. Each adapter variant offers distinct architectural characteristics and capabilities, enabling the model to capture and utilize different levels of abstraction and contextual information from the input data.

$\mathbf{K}$. This hyperparameter determines the number of shots considered for building the visual and textual memory bank. Shots refer to the number of examples available per class in the training set. By adjusting the value of $K$, researchers can control the amount of information captured in the memory bank, potentially influencing the model's ability to generalize and recognize novel instances of the classes.

By carefully selecting and adjusting these hyperparameters, researchers can tailor the behavior and performance of the PROTO-CLIP model to suit their specific research goals. Fine-tuning these parameters empowers researchers to explore different trade-offs and discover optimal configurations that maximize classification accuracy, generalization capabilities, and efficiency.

## 2 Extended Ablation Study

| Adapter | Train Text Memory | Top-1 Accuracy | $\Psi$ |
|---|---|---|---|
| MLP | ✗ | **68.75** | **6** |
| MLP | ✓ | 68.75 | 3 |
| 2xConv | ✗ | 65.62 | 12 |
| 2xConv | ✓ | 62.50 | 57 |
| 3xConv | ✗ | 65.62 | 3 |
| 3xConv | ✓ | 68.75 | 1 |

Table 3: Adapter ablation study. Model=PROTO-CLIP-$F$. Dataset=FEWSOL-198 [1]. $K = 16$. $\Psi$ is the number of $\alpha, \beta$ combinations for which the max accuracy was obtained. Based on $\Psi$, MLP without training the textual memory is the best configuration for FEWSOL-198[1]. Out of the 6 best $\alpha, \beta$ combinations, we selected one randomly.

## 3 t-SNE Plot

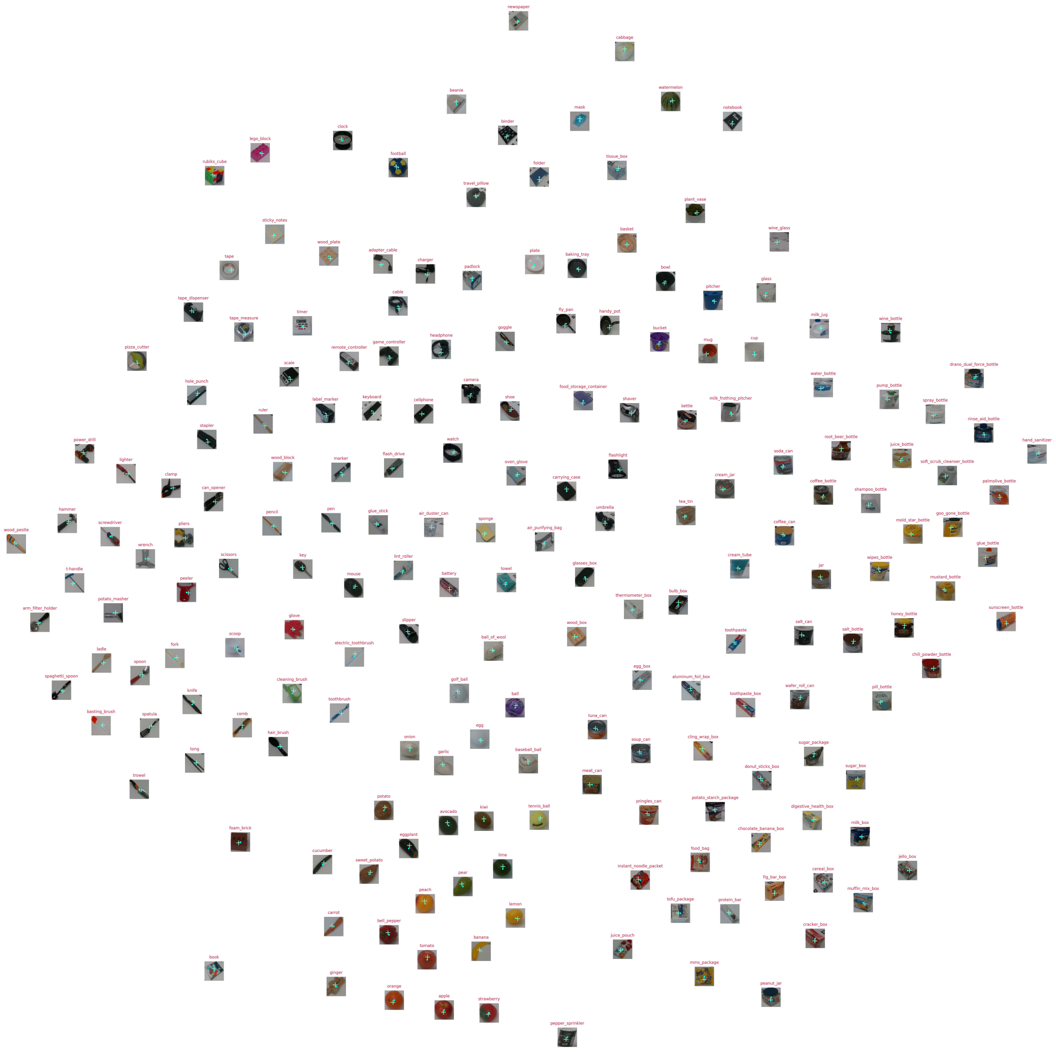

Figure 1: t-SNE [6] plot after training PROTO-CLIP-$F$ on FEWSOL-198 [1].

# 4 Real-World-Testing as in FEWSOL [1]

Following FEWSOL [1], in this experiment, we aim to build a few-shot classification model that works best on real-world perception systems. We train PROTO-CLIP with all real data from the FewSOL dataset, i.e 198 classes and then test the trained model in our lab on the task of joint object segmentation and few-shot classification experiment. The pipeline consists of (i) Collecting RGB-D images from a Fetch mobile manipulator (ii) Unseen object segmentation using UCN [7] and (iii) Few shot classification using PROTO-CLIP. We tested on 32 objects with 4 objects in an image scene and achieved overall top-1 accuracy of 68.75% whereas the baseline Tip-Adapter [3] achieved 65.63%.

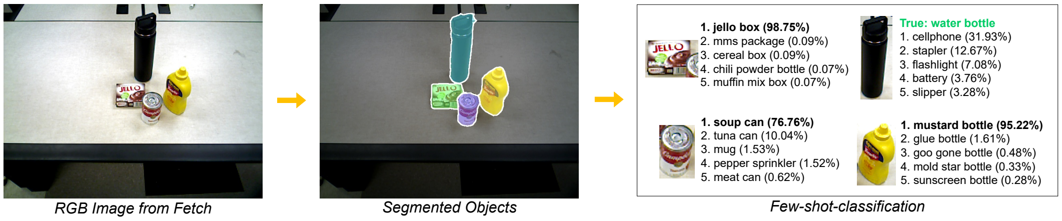


(a) Scene 1

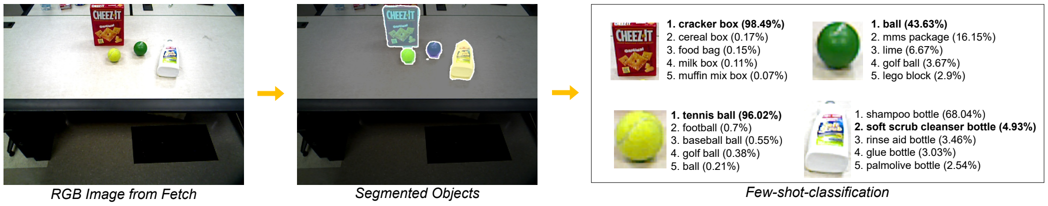


(b) Scene 2

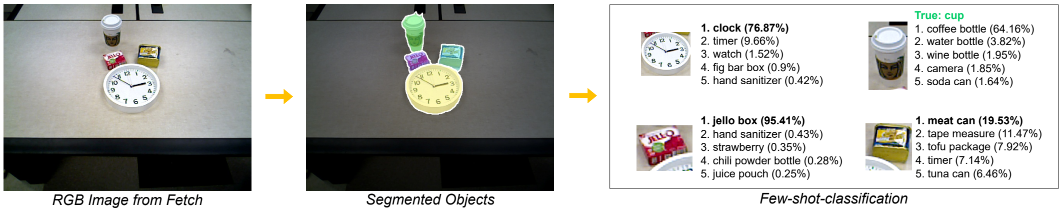


(c) Scene 3

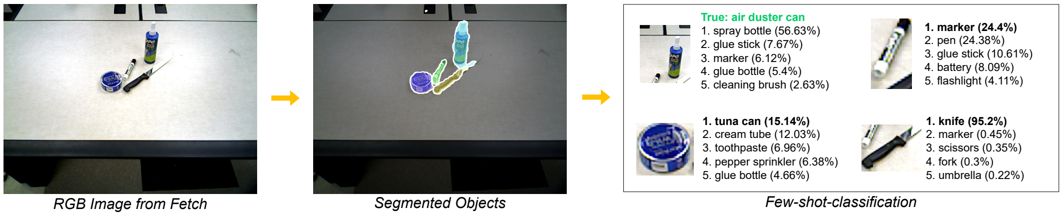


(d) Scene 4

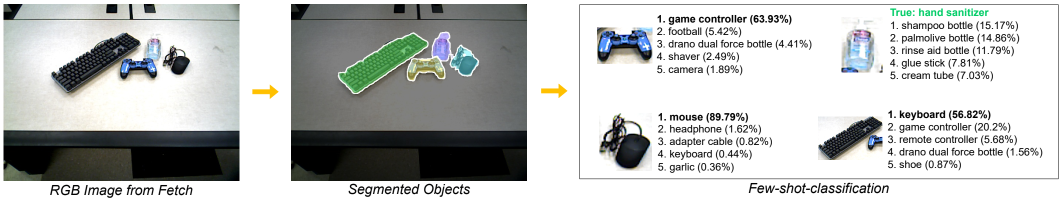


(e) Scene 5

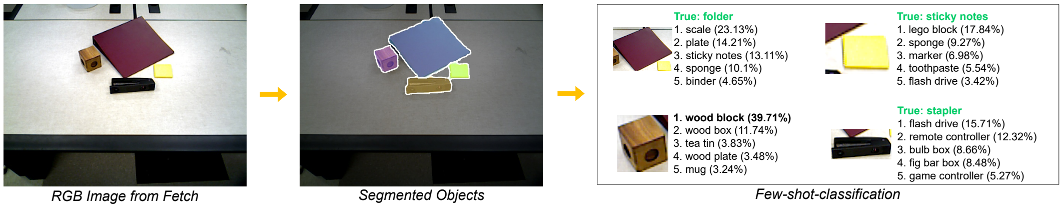


(f) Scene 6

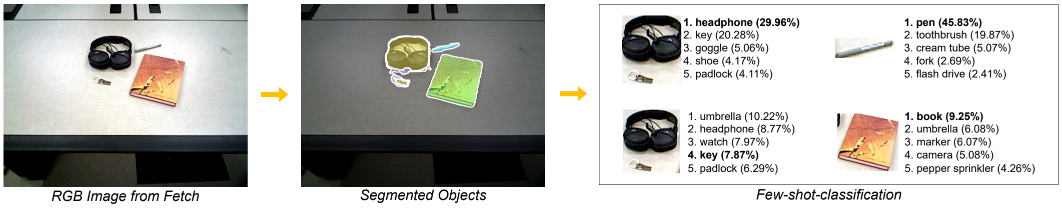


(g) Scene 7

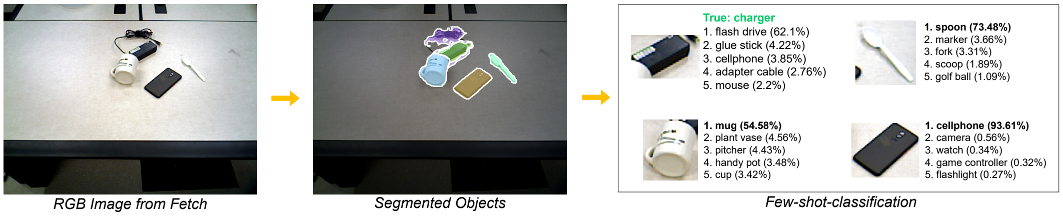


(h) Scene 8

Figure 2: Top-5 predictions for 8 real world scenes (following FewSOL [1]). Here, as indicated in Table 3, the best Proto-CLIP-$F$ model trained on FewSOL-198 dataset has been used.

## 5 Frequently Asked Questions (FAQ)

**Q: How many text prompts have been used in the experiments?**

**A:** All datasets except ImageNet [8] have a single text prompt template. ImageNet uses 7. For comparison purpose, this setting has been borrowed from Tip-Adapter [3]. More text prompts can be used.

**Q: Why has FewSOL been used for real world experiments?**

**A:** For a robot to work in human environments like kitchen, living room etc., it has to interact with various daily objects. FewSOL [1] comes in handy when thinking of learning good representations of daily objects for manipulation tasks. Hence, we chose to experiments with FewSOL.

**Q: Describe the real-world experiments and its outcomes?**

**A:** Following the approach taken in FewSOL [1], we have conducted a comprehensive study involving 32 real-world objects. Our method achieved top-1 accuracy of 68.75%, while Tip-Adapter demonstrates a top-1 accuracy of 65.63%. The model used was trained on FewSOL-198. For a detailed analysis, kindly refer to the appendix section 4. Since the experiments have an external dependency on a custom segmentation method, the quality of segmentation also affects the classification performance. Although we conjecture that more classes could make the classification problem difficult, the current performance of Proto-CLIP makes room for healthy classification and future research. Moreover, we have also executed four real-world experiments focusing on user-command-oriented grasping. These experiments utilized Proto-CLIP predictions and involved four objects each time, with a total of 16 objects placed on a tabletop. The supplementary videos

have been updated with video evidence showcasing the efficacy of our approach. We invite you to review these materials at your convenience. Few key classifications during real world experiments:

- **Instance level:** Different colored bell peppers identified correctly
- **Fine grained:** E.g. Lime vs lemon identified correctly
- **Clutter:** E.g. Scissors on top of umbrella identified correctly

**Q: Any specific observations during inference?**

**A:** Object segmentation and orientation matters. Segmentation is more important as in clutter scenes a bad segmentation can cause problems in classification. Moreover, lighting conditions also play a key role as it impacts classification of shiny objects.

**Q: What are some potential explanations for the difference in behavior between Tip-Adapter and PROTO-CLIP?**

**A:** We think that the behaviour difference is due to the mechanisms that are employed in each settings. Tip-Adapter works by computing support query affinity and then comparing the closeness to the possible classes in textual form which in turn helps in generating the probability distribution for classification. Proto-CLIP on the other hand utilizes the prototypes build from the visual and textual memory banks learned during few shot training and then classifies the incoming query image based on the probability distribution created by the contribution of visual and textual prototypes w.r.t. to the given query image.

**Q: Why the proposed method perform better when K=4, 8, or 16?**

**A:** The enhanced performance of our proposed PROTO-CLIP method can be attributed to its reliance on robust image and textual prototypes, which subsequently leads to improved classification accuracy. In our approach, each embedding within the visual memory bank is computed through multiple augmentations (typically around 10) of a specific image sample. While we did indeed explore the use of augmentations, we found that the inclusion of a greater number of sample images yielded superior outcomes. We hold the perspective that a larger quantity of high-quality samples introduces a richer array of information encompassing texture, lighting, orientation, color, and shapes. This wealth of information significantly contributes to the establishment of more resilient prototypes, thereby fortifying the entire classification process.

**Q: How the proposed and baseline methods perform differently across different datasets?**

**A:** In extremely low shot scenarios, e.g. $K = 1$, PROTO-CLIP variants show competing results w.r.t. the baseline Tip-Adapter [3]. As K increases, PROTO-CLIP starts to show promising results by outperforming the baseline in more datasets.

- $K = 2$, outperforms on $5/12$.
- $K = 4$, outperforms on $7/12$.
- $K = 8$, outperforms on $11/12$ and on par with the remaining one dataset.
- $K = 16$, outperforms on $10/12$ and on par with the remaining two datasets; which shows that more shots might not be good for some datasets.

Hence, it wouldn't hurt to say that different datasets have different needs which can be attributed to its properties.

**Q: What are some of the limitation of PROTO-CLIP?**

**A:** A hyperparameter grid search is necessary for each new dataset, following the methodology of Tip-Adapter. This requirement applies to every combination of the new dataset and the backbone. Embracing the diversity of datasets, our system thrives on the need for different set-ups. When encountering a new dataset, we actively compare the effectiveness of $F$ and $F\text{-}Q^T$ to determine the optimal choice. This dynamic approach transforms the potential weakness into a strength, allowing us to adapt and maximize performance for every unique dataset. During our observations, we discovered that data transformations play a crucial role in building the memory model.

**Q: What is the requirement of PROTO-CLIP when we have SAM [9]?**

**A:** SAM [9] presents a promising approach, although it is not without its limitations. It necessitates the provision of prompts (e.g., Points, Bounding Boxes, Text), or alternatively, the segmentation of all elements within an image. In the former scenario, utilizing any of the prompts aside from textual cues requires the incorporation of heuristics or well-trained models to get reasonable point or bounding boxes to avoid inadvertent area mask predictions. Addressing how to accomplish this in the absence of human input is a distinct question. Regarding text prompts, the SAM paper itself acknowledges its status as a proof of concept. SAM relies on CLIP embeddings when employing text prompts, yet the provided sample results also fall short. To achieve reasonably accurate predictions, supplementary prompts like points or bounding boxes are employed alongside text prompts. In the latter case, where complete image segmentation is pursued, additional post-processing steps are essential to obtain pertinent masks from the generated outputs pertaining to over segmentation, under segmentation and unwanted masks issue. Consequently, while SAM stands as an impressive model, its direct application to robotics use cases is not straightforward; it necessitates integration within a pipeline arrangement. In our endeavors, we incorporated SAM in a cluttered scene setup, yet the outcomes were less than satisfactory. Therefore, we propose that a lightweight model such as ours could potentially enhance SAM's predictions or synergize with analogous methodologies, ultimately bolstering downstream robotic tasks like manipulation or control. Please see the following Study on SAM [2].

# 6 A Study w.r.t. SAM [2]

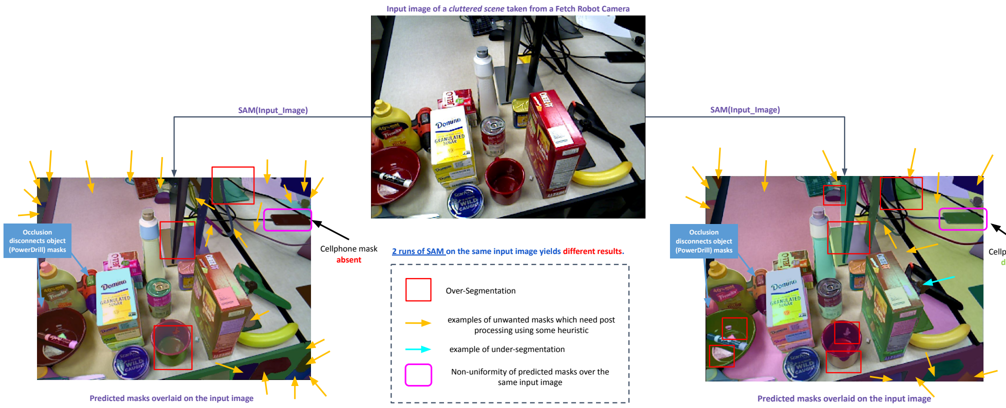


Figure 3: Execution of SAM [2] on a sample real world clutter scene created in our lab.

Although the Segment Anything Model (SAM) [2] is a great method for segmentation, we feel that it's too early to show good performance in robotics context. Clutter scene as shown in Fig. 3 is a prominent example of a robotics environment. A robot will encounter objects in a cluttered scene more often than clean ones. As we can see here, 2 runs of SAM on the same input image yield different results. There is over-segmentation as well as under-segmentation. Occlusion breaks the object connectivity and the masks generated are disjoint. There are several unwanted masks that need post-processing based on some heuristic in absence of a human. Here, we have used the segment

entire image functionality. In order to use the prompt feature of SAM, we need a point location or bounding box as prompt which is possible in presence of a human or some mechanism that can yield good intended masks. In absence of a human, some estimation or approximation method needs to be used. Thus, directly applying SAM in robotics might not be a good option. However, it can act as a module in a large robotic pipeline for downstream tasks.

Our PROTO-CLIP model can join forces with the predictions of SAM for better classification of the detected masks (after removing the unwanted masks). Unseen object segmentation methods like [10, 11, 12, 13] are specifically targetted towards finding masks of **novel objects** in different scenes hence we believe that they have an upper hand in robotics context as they can aid robot manipulation tasks on novel objects. Fig. 4 (Scene:1-8) show the predictions of SAM [2] vs UCN [11]. PROTO-CLIP can be used in combination with any of these for downstream tasks involving vision-language modalities.

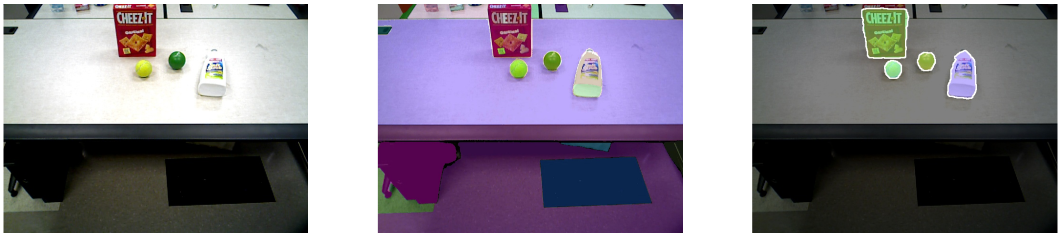

*RGB Image from Fetch* | *SAM Segmentation* | *UCN Segmentation*

**Scene-1**

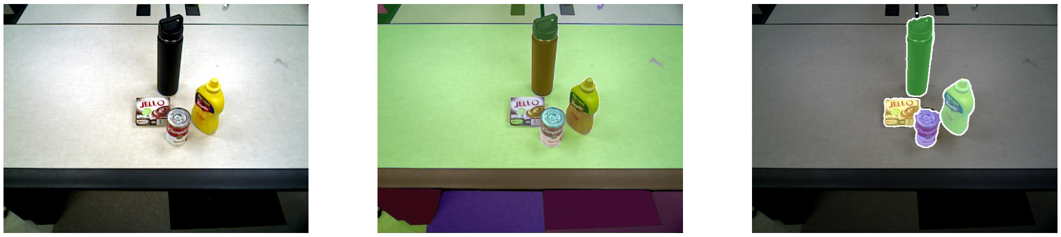

*RGB Image from Fetch* | *SAM Segmentation* | *UCN Segmentation*

**Scene-2**

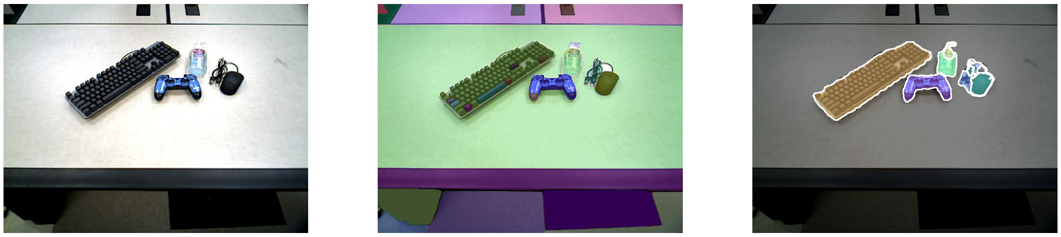

*RGB Image from Fetch* | *SAM Segmentation* | *UCN Segmentation*

**Scene-3**

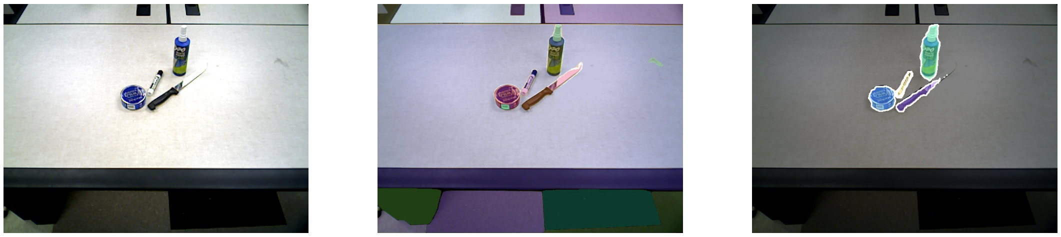

*RGB Image from Fetch* | *SAM Segmentation* | *UCN Segmentation*

**Scene-4**

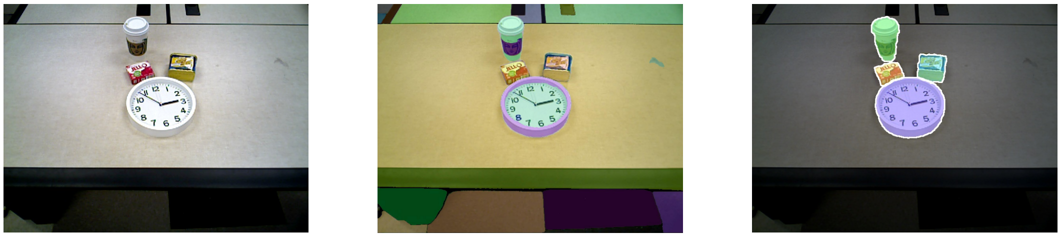

RGB Image from Fetch | SAM Segmentation | UCN Segmentation

**Scene-5**

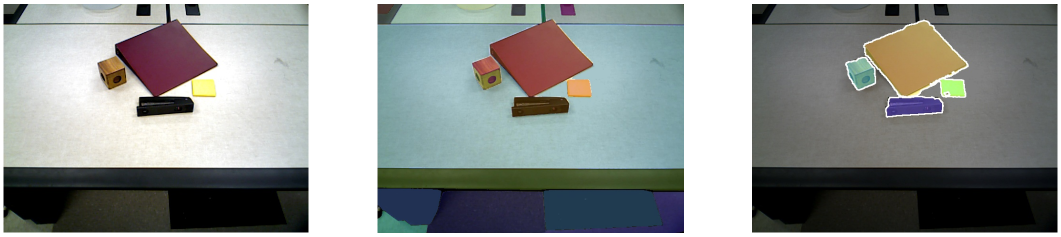

RGB Image from Fetch | SAM Segmentation | UCN Segmentation

**Scene-6**

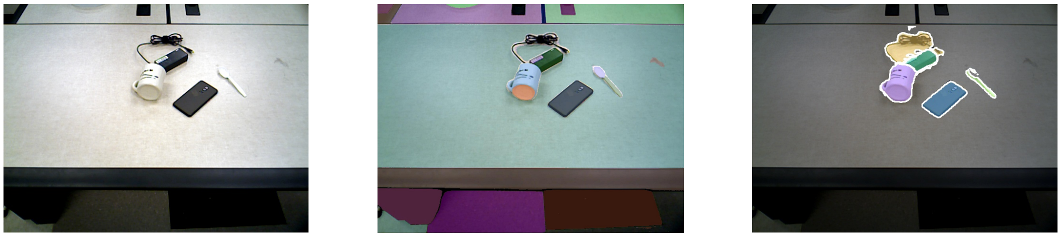

RGB Image from Fetch | SAM Segmentation | UCN Segmentation

**Scene-7**

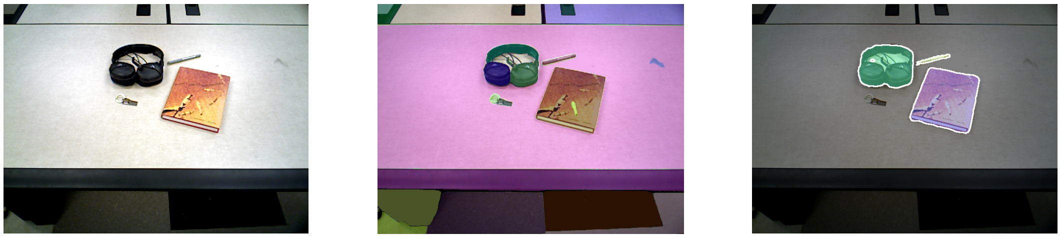

RGB Image from Fetch | SAM Segmentation | UCN Segmentation

**Scene-8**

Figure 4: 8 real world scenes as used in FewSOL [1]. SAM [2] predicts masks for the entire image in the absence of prompts like points or bounding boxes. Corresponding UCN [11] predictions which are far better in targeting object-centric masks.

## References


[1] J. J. P, Y.-W. Chao, and Y. Xiang. Fewsol: A dataset for few-shot object learning in robotic environments. In *2023 IEEE International Conference on Robotics and Automation (ICRA)*, pages 9140–9146, 2023. doi:10.1109/ICRA48891.2023.10161143.

[2] A. Kirillov, E. Mintun, N. Ravi, H. Mao, C. Rolland, L. Gustafson, T. Xiao, S. Whitehead, A. C. Berg, W.-Y. Lo, P. Dollár, and R. Girshick. Segment anything. *arXiv:2304.02643*, 2023.

[3] R. Zhang, Z. Wei, R. Fang, P. Gao, K. Li, J. Dai, Y. Qiao, and H. Li. Tip-adapter: Training-free adaption of clip for few-shot classification. *arXiv preprint arXiv:2207.09519*, 2022.

[4] A. Radford, J. W. Kim, C. Hallacy, A. Ramesh, G. Goh, S. Agarwal, G. Sastry, A. Askell, P. Mishkin, J. Clark, et al. Learning transferable visual models from natural language supervision. In *International Conference on Machine Learning*, pages 8748–8763, 2021.

[5] G. Hinton, O. Vinyals, and J. Dean. Distilling the knowledge in a neural network. *arXiv preprint arXiv:1503.02531*, 2015.

[6] L. Van Der Maaten. Accelerating t-sne using tree-based algorithms. *The journal of machine learning research*, 15(1):3221–3245, 2014.

[7] Y. Xiang, C. Xie, A. Mousavian, and D. Fox. Learning RGB-D feature embeddings for unseen object instance segmentation. In *Conference on Robot Learning (CoRL)*, pages 461–470, 2021.

[8] J. Deng, W. Dong, R. Socher, L.-J. Li, K. Li, and L. Fei-Fei. ImageNet: A large-scale hierarchical image database. In *IEEE Conference on Computer Vision and Pattern Recognition (CVPR)*, pages 248–255, 2009.

[9] A. Kirillov, E. Mintun, N. Ravi, H. Mao, C. Rolland, L. Gustafson, T. Xiao, S. Whitehead, A. C. Berg, W.-Y. Lo, P. Dollár, and R. Girshick. Segment anything. *arXiv:2304.02643*, 2023.

[10] C. Xie, Y. Xiang, A. Mousavian, and D. Fox. Unseen object instance segmentation for robotic environments. *IEEE Transactions on Robotics*, 37(5):1343–1359, 2021.

[11] Y. Xiang, C. Xie, A. Mousavian, and D. Fox. Learning rgb-d feature embeddings for unseen object instance segmentation. In J. Kober, F. Ramos, and C. Tomlin, editors, *Proceedings of the 2020 Conference on Robot Learning*, volume 155 of *Proceedings of Machine Learning Research*, pages 461–470. PMLR, 16–18 Nov 2021. URL https://proceedings.mlr.press/v155/xiang21a.html.

[12] C. Xie, Y. Xiang, A. Mousavian, and D. Fox. The best of both modes: Separately leveraging rgb and depth for unseen object instance segmentation. In *Conference on robot learning*, pages 1369–1378. PMLR, 2020.

[13] Y. Lu, Y. Chen, N. Ruozzi, and Y. Xiang. Mean shift mask transformer for unseen object instance segmentation, 2023.
